# Supplementary material for: An Experimental Comparison of Floating Base Estimators for Humanoid Robots with Flat Feet
Source: arXiv:2205.07765 source file (2022-05-16)
Supplement: Supplementary file 1 [file appendix.tex]

\appendix
